# Supplementary material for: Polyhedral Collision Detection via Vertex Enumeration
Source: arXiv:2501.13201 source file (2025-03-10)
Supplement: Supplementary file 1 [file appendix.tex]

Given a closed convex set, which can be bounded or unbounded, as follows:
 \begin{equation} \label{eq:convex_set}
     h(p) \ge 0,
 \end{equation}
where $h(p)$ is a concave function.

We define a parameterized closed convex set with a parameter  $\alpha \in [-1, \infty)$ as follows:
\begin{equation} \label{eq:para_convex_set}
     h(p+\alpha (c-p^*))+\alpha h^* \ge 0,
\end{equation}
where $c$ can be any point, $p^*$ is a point that satisfies \ref{eq:convex_set}, and $h^*=h(p^*)$. 
This parameterized set is equivalent to \ref{eq:convex_set} when $\alpha=0$, and includes the point $p=c$ when $\alpha=-1$.

Intuitively, the first term in \ref{eq:para_convex_set} "shifts" the original set so that the position of $p^*$ relative to the original set becomes the position of $c$ relative to the new set as $\alpha$ changes from $0$ to $-1$. The second term "scales" this set with factor $\alpha$. Notice that $h^*$ is always non-negative, so $\alpha > 0$ will increase the set size, and $\alpha < 0$ will decrease the set size.

If $h(p)$ has a maximum point, let $p^*$ be this maximum point, then $h^*$ is the maximum value. When $\alpha=-1$, \ref{eq:para_convex_set} becomes $h(p-c+p^*)-h^* \ge 0$, which has a unique solution $p=c$. Thus, the set \ref{eq:para_convex_set} deflates from the original set to a singleton $\{c\}$ as $\alpha$ changes from $0$ to $-1$.
If $h(p)$ is affine, $p^*$ and $h^*$ are eliminated regardless of the choice of $p^*$, and \ref{eq:para_convex_set} simplifies to $h(p)+\alpha h(c) \ge 0$. When $\alpha=-1$, the original set becomes a half-space whose boundary passes through the point $c$. Thus, the set \ref{eq:para_convex_set} shifts from the original half-space to a half-space whose boundary intersects $c$ as $\alpha$ changes from $0$ to $-1$.

Next, consider a convex object $\mathcal{O}$ consisting of multiple constraints discussed above, defined as in \ref{eq:obj}, and a scaled object $\mathcal{O}(\alpha)$ defined similarly to \ref{eq:obj_xt_alpha} (ignoring $x_t$). 
If at least one concave function $h_j$ has a maximum point $p_j^*$, the convex set corresponding to $h_j$ becomes a singleton $\{c\}$ when $\alpha=-1$, also included by half-spaces defined by affine constraints. Thus, the intersection of these constraints, i.e., the object, also becomes the singleton $\{c\}$.
If all constraints are affine, when $\alpha=-1$, the boundaries of these shifted half-spaces intersects at the same point $c$. Thus, the only point satisfying all constraints is $c$, meaning the object becomes a singleton $\{c\}$.
